# Supplementary material for: Quantum transport of vortex electrons in bending magnets and circular accelerators
Source: arXiv:2611.08010 source file (2026-11-05)
Supplement: Supplementary file 14 [file supplement_references.tex]

\begin{thebibliography}{99}
\bibitem{Karlovets2021}D. Karlovets, Vortex particles in axially symmetric fields and applications of the quantum Busch theorem, \href{https://doi.org/10.1088/1367-2630/abeacc}{New J. Phys. \textbf{23}, 033048 (2021)}.
\bibitem{BagrovBelovKondrateva1994}{{{V. G. Bagrov, V. V. Belov, and M. F. Kondrat'eva, The semiclassical approximation in quantum mechanics. A new approach, \href{https://doi.org/10.1007/BF01015121}{Theor. Math. Phys. \textbf{98}, 34 (1994)}.}}}
\bibitem{BagrovBelovTrifonov2005}{{V. G. Bagrov, V. V. Belov, and A. Yu. Trifonov, \textit{Methods of Mathematical Physics: Asymptotic Methods} (Tomsk Polytechnic University Press, Tomsk, 2005) (in Russian).}}
\bibitem{BagrovBelovTrifonov2006}{{V. G. Bagrov, V. V. Belov, and A. Yu. Trifonov, \textit{Methods of Mathematical Physics: Asymptotic Methods in Relativistic Quantum Mechanics} (Tomsk Polytechnic University Press, Tomsk, 2006) (in Russian).}}
\bibitem{BagrovBelovMaslov1989}{V. G. Bagrov, V. V. Belov, and V. P. Maslov, The method of quasiclassical trajectory-coherent states in the theory of spontaneous electron radiation, Sov. Phys. Dokl. \textbf{34}, 809--811 (1989) [\href{https://www.mathnet.ru/eng/dan6978}{Dokl. Akad. Nauk SSSR \textbf{308}, 88--91 (1989)}].}
\bibitem{BagrovBelovTernov1983}{{{V. G. Bagrov, V. V. Belov, and I. M. Ternov, Quasiclassical trajectory-coherent states of a particle in an arbitrary electromagnetic field, \href{https://doi.org/10.1063/1.525666}{J. Math. Phys. \textbf{24}, 2855 (1983)}.}}}
\bibitem{BagrovBelovTrifonov1993}{{V. G. Bagrov, V. V. Belov, and A. Yu. Trifonov, Theory of spontaneous radiation by electrons in a trajectory-coherent approximation, \href{https://doi.org/10.1088/0305-4470/26/22/038}{J. Phys. A: Math. Gen. \textbf{26}, 6431 (1993)}.}}
\bibitem{BagrovBelovTrifonov1996}{{{V. G. Bagrov, V. V. Belov, and A. Yu. Trifonov, Semiclassical trajectory-coherent approximation in quantum mechanics I. High-order corrections to multidimensional time-dependent equations of Schr\"odinger type, \href{https://doi.org/10.1006/aphy.1996.0027}{Ann. Phys. \textbf{246}, 231 (1996)}.}}}
\bibitem{Maslov1994}{V. P. Maslov, \href{https://doi.org/10.1007/978-3-0348-8536-2}{\textit{The Complex WKB Method for Nonlinear Equations I: Linear Theory}} (Birkh\"auser, Basel, 1994).}
\bibitem{GrilloSpectrum2017}{{V. Grillo, A. H. Tavabi, F. Venturi, H. Larocque, R. Balboni, G. C. Gazzadi, S. Frabboni, P.-H. Lu, E. Mafakheri, F. Bouchard, R. E. Dunin-Borkowski, R. W. Boyd, M. P. J. Lavery, M. J. Padgett, and E. Karimi, Measuring the orbital angular momentum spectrum of an electron beam, \href{https://doi.org/10.1038/ncomms15536}{Nat. Commun. \textbf{8}, 15536 (2017)}.}}
\bibitem{MaksimovDiagnostic2025}{{M. Maksimov, N. Borodin, D. Kargina, D. Naumov, and D. Karlovets, Diffraction by circular and triangular apertures as a diagnostic tool of twisted matter waves, \href{https://doi.org/10.1103/z2rs-2ryl}{Phys. Rev. A \textbf{112}, 062823 (2025)}.}}
\bibitem{JINRphoto}{{M. A. Nozdrin (private communication).}}
\bibitem{Roura}{{A. Roura, Gravitational redshift in quantum-clock interferometry, \href{https://doi.org/10.1103/PhysRevX.10.021014}{Phys. Rev. X \textbf{10}, 021014 (2020)}.}}
\bibitem{OST}{Yu. N. Obukhov, A. J. Silenko, and O. V. Teryaev, Spin in an arbitrary gravitational field, \href{https://doi.org/10.1103/PhysRevD.88.084014}{Phys. Rev. D \textbf{88}, 084014 (2013)}.}
\bibitem{Hillery}{{{M. Hillery, R. F. O'Connell, M. O. Scully, and E. P. Wigner, Distribution functions in physics: Fundamentals, \href{https://doi.org/10.1016/0370-1573(84)90160-1}{Phys. Rep. \textbf{106}, 121 (1984)}.}}}
\bibitem{GatalinaBaturin2026}{{S. V. Gatalina and S. S. Baturin, Fringe-field-induced spin-orbit angular momentum mixing of twisted electrons, \href{https://doi.org/10.1103/97y1-jx9b}{Phys. Rev. A \textbf{114}, 022828 (2026)}.}}
\bibitem{Greenshields2014}{C. R. Greenshields, R. L. Stamps, S. Franke-Arnold, and S. M. Barnett, Is the angular momentum of an electron conserved in a uniform magnetic field?, \href{https://doi.org/10.1103/PhysRevLett.113.240404}{Phys. Rev. Lett. \textbf{113}, 240404 (2014)}.}
\bibitem{Silenko2017}{A. J. Silenko, P. Zhang, and L. Zou, Manipulating twisted electron beams, \href{https://doi.org/10.1103/PhysRevLett.119.243903}{Phys. Rev. Lett. \textbf{119}, 243903 (2017)}.}
\bibitem{Silenko2018}{A. J. Silenko, P. Zhang, and L. Zou, Relativistic quantum dynamics of twisted electron beams in arbitrary electric and magnetic fields, \href{https://doi.org/10.1103/PhysRevLett.121.043202}{Phys. Rev. Lett. \textbf{121}, 043202 (2018)}.}
\bibitem{Karlovets2026}{D. Karlovets, D. Grosman, and I. Pavlov, Angular momentum dynamics of vortex particles in accelerators, \href{https://doi.org/10.1103/gsrz-cscl}{Phys. Rev. Lett. \textbf{136}, 085002 (2026)}.}
\bibitem{Bliokh2026}{K. Y. Bliokh, Expectation Pauli--Lubanski vector and intrinsic angular momentum of relativistic wavepackets, \href{https://doi.org/10.1088/1367-2630/ae98a5}{New J. Phys. \textbf{28}, 094501 (2026)}.}
\bibitem{BMT}{{{V. Bargmann, L. Michel, and V. L. Telegdi, Precession of the polarization of particles moving in a homogeneous electromagnetic field, \href{https://doi.org/10.1103/PhysRevLett.2.435}{Phys. Rev. Lett. \textbf{2}, 435 (1959)}.}}}
\bibitem{ManePolarized2005}{{{S. R. Mane, Yu. M. Shatunov, and K. Yokoya, Spin-polarized charged particle beams in high-energy accelerators, \href{https://doi.org/10.1088/0034-4885/68/9/R01}{Rep. Prog. Phys. \textbf{68}, 1997 (2005)}.}}}
\bibitem{ManeSnakes2005}{{S. R. Mane, Yu. M. Shatunov, and K. Yokoya, Siberian snakes in high-energy accelerators, \href{https://doi.org/10.1088/0954-3899/31/9/R01}{J. Phys. G: Nucl. Part. Phys. \textbf{31}, R151 (2005)}.}}
\bibitem{SilenkoTeryaevSnake2019}{{A. J. Silenko and O. V. Teryaev, Siberian snake-like behavior for an orbital polarization of a beam of twisted (vortex) electrons, \href{https://doi.org/10.1134/S1547477119020134}{Phys. Part. Nucl. Lett. \textbf{16}, 77 (2019)}.}}
\bibitem{SizykhSolenoid2024}G. K. Sizykh, A. D. Chaikovskaia, D. V. Grosman, I. I. Pavlov, and D. V. Karlovets, Transmission of vortex electrons through a solenoid, \href{https://doi.org/10.1103/PhysRevA.109.L040201}{Phys. Rev. A \textbf{109}, L040201 (2024)}.
\bibitem{HwangLee2015}{K. Hwang and S. Y. Lee, Dipole fringe field thin map for compact synchrotrons, \href{https://doi.org/10.1103/PhysRevSTAB.18.122401}{Phys. Rev. ST Accel. Beams \textbf{18}, 122401 (2015)}.}
\bibitem{Robertson1934}{{H. P. Robertson, An indeterminacy relation for several observables and its classical interpretation, \href{https://doi.org/10.1103/PhysRev.46.794}{Phys. Rev. \textbf{46}, 794 (1934)}.}}
\bibitem{Gallatin}G. M. Gallatin and B. McMorran, Propagation of vortex electron wave functions in a magnetic field, \href{https://doi.org/10.1103/PhysRevA.86.012701}{Phys. Rev. A \textbf{86}, 012701 (2012)}.
\bibitem{KarlovetsSerbo2020}D. V. Karlovets and V. G. Serbo, Effects of the transverse coherence length in relativistic collisions, \href{https://doi.org/10.1103/PhysRevD.101.076009}{Phys. Rev. D \textbf{101}, 076009 (2020)}.
\bibitem{Littlejohn1986}{{R. G. Littlejohn, The semiclassical evolution of wave packets, \href{https://doi.org/10.1016/0370-1573(86)90103-1}{Phys. Rep. \textbf{138}, 193 (1986)}.}}
\bibitem{Folland1989}{G. B. Folland, \textit{Harmonic Analysis in Phase Space} (Princeton University Press, Princeton, 1989).}
\bibitem{deGosson2011}{M. A. de Gosson, \href{https://doi.org/10.1007/978-3-7643-9992-4}{\textit{Symplectic Methods in Harmonic Analysis and in Mathematical Physics}} (Birkh\"auser, Basel, 2011).}
\bibitem{BliokhNori2012}K. Y. Bliokh and F. Nori, Spatiotemporal vortex beams and angular momentum, \href{https://doi.org/10.1103/PhysRevA.86.033824}{Phys. Rev. A \textbf{86}, 033824 (2012)}.
\bibitem{Dennis2006}{{{M. R. Dennis, Rows of optical vortices from elliptically perturbing a high-order beam, \href{https://doi.org/10.1364/OL.31.001325}{Opt. Lett. \textbf{31}, 1325 (2006)}.}}}
\bibitem{IvanovSerbo2011}I. P. Ivanov and V. G. Serbo, Scattering of twisted particles: Extension to wave packets and orbital helicity, \href{https://doi.org/10.1103/PhysRevA.84.033804}{Phys. Rev. A \textbf{84}, 033804 (2011)}; \href{https://doi.org/10.1103/PhysRevA.84.069906}{\textbf{84}, 069906(E) (2011)}.
\bibitem{IvanovHelicity2012}I. P. Ivanov, Creation of two vortex-entangled beams in a vortex-beam collision with a plane wave, \href{https://doi.org/10.1103/PhysRevA.85.033813}{Phys. Rev. A \textbf{85}, 033813 (2012)}.
\bibitem{IMP2024}{{Z. Yang \textit{et al.}, Stable acceleration of a LHe-Free Nb$_3$Sn demo SRF e-linac, \href{https://doi.org/10.1088/1361-6668/ad9998}{Supercond. Sci. Technol. \textbf{38}, 015009 (2025)}.}}
\bibitem{MADX}{{MAD-X Collaboration, \href{https://github.com/MethodicalAcceleratorDesign/MAD-X-User-Manual/blob/master/elements.tex}{MAD-X User Manual}, FINT and HGAP definitions (accessed October 10, 2026).}}
\bibitem{JINRcurrent}{{{A. S. Dyatlov, V. V. Kobets, A. E. Levichev, M. V. Maksimov, D. A. Nikiforov, M. A. Nozdrin, K. Popov, K. A. Sibiryakova, K. E. Yunenko, and D. V. Karlovets, Classical and quantum beam dynamics simulation of the RF photoinjector test bench, \href{https://arxiv.org/abs/2509.00732v4}{arXiv:2509.00732v4}.}}}
\bibitem{JINRmagnets}{{{{O. L. Seroshtanov, V. V. Kobets, A. N. Trifonov, and A. A. Ulankin, Development of a magnetic system for parallel electron beam transfer in the LINAC-200 accelerator, \href{https://www1.jinr.ru/Pepan_letters/panl_2025_4/32_Seroshtanov_rus_utf8.pdf}{Pis'ma v EChAYa \textbf{22}, 765 (2025)} [\href{https://doi.org/10.1134/S1547477125700578}{Phys. Part. Nucl. Lett. \textbf{22}, 783 (2025)}].}}}}
\bibitem{BNL}{Brookhaven National Laboratory, \href{https://www.bnl.gov/atf/beamlines/parameters.php}{Accelerator Test Facility: Beamline Parameters} (accessed October 10, 2026).}
\bibitem{BNLcurrent}{Brookhaven National Laboratory, \href{https://www.bnl.gov/atf/capabilities/electron-beam-systems.php}{Accelerator Test Facility: Electron Beam Systems} (accessed October 10, 2026).}
\bibitem{MESA}{{F. Hug, \href{https://indico.classe.cornell.edu/event/2018/contributions/1831/attachments/1431/1935/Hug-MESA_Overview_ERL_2022.pdf}{MESA overview}, ERL 2022 (2022), slide 24.}}
\bibitem{ELBEchicane}{{V. Verzilov, \href{https://indico.triumf.ca/event/510/contributions/5462/attachments/3772/5059/FEL_Workshop_Triumf_Mar.2024.pdf}{A Test Bed for Intense THz Radiation at the ARIEL E-linac}, IR-FEL Workshop, TRIUMF (March 19, 2024), slide 12.}}
\bibitem{JINR}{{Joint Institute for Nuclear Research, \href{https://www.jinr.ru/posts/new-dlnp-jinr-main-facility-launched/}{New DLNP JINR main facility launched} (February 17, 2025).}}
\bibitem{IMPdiagnostics}{{{Y. M. Chu \textit{et al.}, Measurement of beam energy characteristics at the LHe-free Nb$_3$Sn demo SRF e-linac, in \href{https://doi.org/10.18429/JACoW-IBIC2024-THP66}{\textit{Proceedings of the 13th International Beam Instrumentation Conference (IBIC2024)}, Beijing, China (JACoW Publishing, Geneva, 2024)}, p.~633.}}}
\bibitem{MESAcurrent}{{E. Khidr, F. Hug, and F. Schliessmann, Improving energy spread of MESA beam in ERL operation, in \href{https://www.ipac26.org/prepress/doi/jacow-ipac2026-wep5023/index.html}{\textit{Proceedings of the 17th International Particle Accelerator Conference (IPAC2026)}, Deauville, France (JACoW Publishing, Geneva, 2026)}, pp.~3109--3112.}}
\bibitem{PERLE}{{R. Abukeshek, \href{https://indico.cern.ch/event/1417048/contributions/6101849/attachments/2927995/5141160/16092024\%20perle_collaboration_cern_Rasha\%20.pdf}{Magnet Design and Optics Misalignment}, PERLE Collaboration Meeting, CERN (September 17, 2024), slides 3--5.}}
\bibitem{PERLEcurrent}{{M. Baylac, \href{https://isas.ijclab.in2p3.fr/news/2026/05/28/1st-perle-beam.html}{First PERLE beam}, iSAS/IJCLab (May 28, 2026).}}
\bibitem{IOTA}{{A. Romanov, G. Stancari, J. Santucci, and J. Jarvis, Analysis of the elliptic integrable non-linear system in IOTA using tracking of a single electron, in \href{https://doi.org/10.18429/JACoW-NAPAC2025-TUP008}{\textit{Proceedings of the 6th North American Particle Accelerator Conference (NAPAC2025)}, Sacramento, CA (JACoW Publishing, Geneva, 2026)}, p.~361.}}
\bibitem{IOTAfacility}{{{{S. Antipov \textit{et al.}, IOTA (Integrable Optics Test Accelerator): Facility and experimental beam physics program, \href{https://doi.org/10.1088/1748-0221/12/03/T03002}{J. Instrum. \textbf{12}, T03002 (2017)}.}}}}
\bibitem{DELTA}{{TU Dortmund University, \href{https://delta.tu-dortmund.de/en/newsdetail/operating-delta-with-a-single-electron-33779/}{Operating DELTA with a single electron} (February 18, 2023).}}
\bibitem{BaturinTransport2026}{S. S. Baturin, State-resolved quantum transport of vortex electrons in accelerators, \href{https://arxiv.org/abs/2608.11934v2}{arXiv:2608.11934v2}.}
\bibitem{MIRRORCLE2006}{{{H. Yamada, D. Hasegawa, M. Morita, T. Hirai, and M. Sasaki, Phase contrast imaging realized by the tabletop synchrotron and the way to portable synchrotron for medical diagnosis, \href{https://www.jstage.jst.go.jp/article/mit/24/5/24_385/_article}{Med. Imaging Technol. \textbf{24}, 385 (2006)}.}}}
\end{thebibliography}
